# Supplementary material for: Analytic Gradients of Approximate Coupled Cluster Methods with Quadruple Excitations
Source: arXiv:2005.10178 ancillary file (2020-05-20)
Supplement: Supplementary file 1 [file si.pdf]

# Analytic Gradients of Approximate CCSDTQ Methods: Supplemental Information

Devin A. Matthews

*Department of Chemistry, Southern Methodist University, Dallas, TX 75275*

## I. DIMETHYLCARBENE–PROPENE ISOMERIZATION

The geometries of the DMC and propene minima and the isomerization transition state are depicted in Figure 1. Numbered atoms correspond to the numbered bond lengths and angles in Tables I, III, and V. For DMC, $\phi_1/\phi_2$ are the dihedral angles between atoms H2/H3 and H1 along the neighboring C–C bond, while $\phi_3$ is the dihedral angle ∠H1–C–C–C. For propene, the lone dihedral angle $\phi$ is the angle between H2 and H1 along the C–C bond. The six dihedral angles for the transition state are, in numbered order: the angle between H2 and H1 and between H6 and H1 along the neighboring C–C bond, the angles ∠H1–C–C–C, ∠H3–C–C–C, and ∠H4–C–C–C, and finally the angle between H5 and H1 along the C–C1 bond (note that H1 is not proximal to this bond). Also note that the C–H5 bond distance is measured from from the central carbon, not C2, and that its bond angle is ∠H5–C–C2.

The individual errors for all geometric quantities compared to the CCSDTQ values (also listed) are given in Tables I, III, and V for DMC, *g*-TS, and propene, respectively. The errors for the harmonic vibrational frequencies are listed likewise in Tables II, IV, and VI. Rotational constants are given in MHz, bond lengths are in Å, all angles are in degrees, and harmonic frequencies are given in $\text{cm}^{-1}$.

## II. CRIEGEE INTERMEDIATE

The geometry of $CH_2OO$ is planar, and the *cis* hydrogen is labeled as H1. The individual errors for all geometric quantities compared to the CCSDTQ values (also listed) are given in Table VII. The errors for the harmonic vibrational frequencies are listed likewise in Table VIII. Rotational constants are given in MHz, bond lengths are in Å, all angles are in degrees, and harmonic frequencies are given in $\text{cm}^{-1}$.

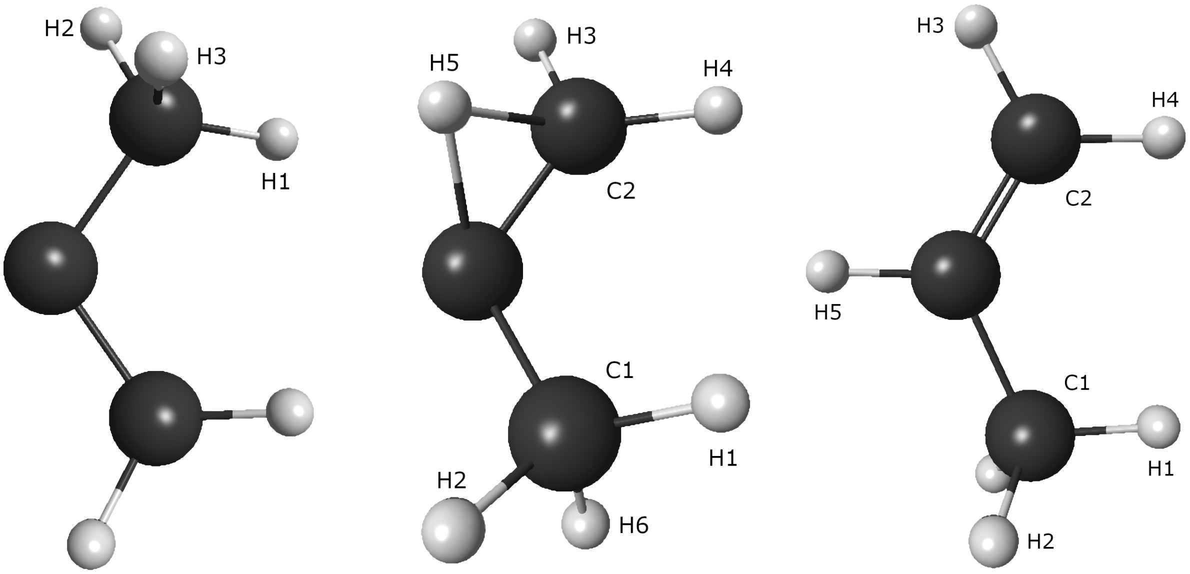


(a) $g$-DMC (b) $g$-TS (c) Propene

Figure 1: Geometries of the DMC and propene minima and the isomerization transition state.

| | (T) | T | (Q) | (Q)/A | (Q)/B | Q-1a | Q-1b | Q-3 | CC4 | Q |
|---|---|---|---|---|---|---|---|---|---|---|
| $A_e$ | 0.03% | 0.02% | -0.01% | 0.00% | 0.00% | 0.01% | 0.00% | 0.01% | 0.00% | 40113.6 |
| $B_e$ | 0.13% | 0.03% | 0.00% | 0.00% | 0.00% | 0.01% | 0.00% | 0.01% | 0.00% | 9259.7 |
| $C_e$ | 0.11% | 0.03% | 0.00% | 0.00% | 0.00% | 0.01% | 0.00% | 0.01% | 0.00% | 8274.0 |
| $r_{\rm CC}$ | -0.0007 | -0.0002 | 0.0000 | 0.0000 | 0.0000 | -0.0001 | 0.0000 | -0.0001 | 0.0000 | 1.4957 |
| $r_{\rm CH1}$ | -0.0002 | -0.0001 | 0.0000 | 0.0000 | 0.0000 | -0.0001 | 0.0000 | -0.0001 | 0.0000 | 1.1050 |
| $r_{\rm CH2}$ | -0.0002 | -0.0001 | 0.0000 | 0.0000 | 0.0000 | -0.0001 | 0.0000 | 0.0000 | 0.0000 | 1.0970 |
| $r_{\rm CH3}$ | -0.0001 | -0.0001 | 0.0000 | 0.0000 | 0.0000 | -0.0001 | 0.0000 | -0.0001 | 0.0000 | 1.1127 |
| $\angle_{\rm CCC}$ | -0.038 | 0.000 | -0.004 | -0.002 | -0.003 | 0.000 | -0.004 | 0.001 | -0.003 | 109.971 |
| $\angle_{\rm CCH1}$ | 0.048 | 0.000 | 0.003 | 0.000 | 0.001 | -0.008 | 0.003 | 0.000 | 0.003 | 117.520 |
| $\angle_{\rm CCH2}$ | 0.031 | 0.002 | 0.001 | 0.001 | 0.001 | -0.007 | 0.002 | -0.001 | 0.002 | 113.785 |
| $\angle_{\rm CCH3}$ | -0.140 | -0.003 | -0.008 | -0.007 | -0.008 | 0.013 | -0.011 | 0.000 | -0.011 | 99.740 |
| $\phi_1$ | 0.129 | -0.006 | 0.009 | 0.003 | 0.005 | -0.028 | 0.008 | -0.004 | 0.009 | 133.010 |
| $\phi_2$ | 0.048 | -0.004 | 0.004 | 0.002 | 0.002 | -0.016 | 0.004 | -0.004 | 0.004 | -114.647 |
| $\phi_3$ | -0.174 | 0.002 | -0.013 | -0.002 | -0.006 | 0.026 | -0.010 | 0.001 | -0.012 | 21.021 |

Table I: $g$-DMC: Geometry.

| | (T) | T | (Q) | (Q)/A | (Q)/B | Q-1a | Q-1b | Q-3 | CC4 | Q |
|---|---|---|---|---|---|---|---|---|---|---|
| $\omega_1$ | 3.04 | 1.08 | -0.10 | 0.05 | -0.01 | 1.12 | 0.01 | 0.61 | -0.04 | 3130.15 |
| $\omega_2$ | 3.31 | 1.57 | -0.14 | 0.12 | 0.03 | 1.79 | 0.04 | 0.87 | -0.01 | 3029.84 |
| $\omega_3$ | 2.35 | 1.33 | -0.13 | 0.09 | 0.01 | 1.90 | -0.04 | 0.80 | -0.09 | 2959.27 |
| $\omega_4$ | 1.90 | 1.16 | -0.08 | 0.01 | -0.02 | 0.83 | 0.00 | 0.43 | -0.04 | 1500.83 |
| $\omega_5$ | 0.95 | 1.09 | -0.15 | 0.01 | -0.04 | 0.93 | -0.05 | 0.42 | -0.07 | 1411.33 |
| $\omega_6$ | 1.32 | 1.33 | -0.16 | -0.01 | -0.06 | 1.05 | -0.06 | 0.49 | -0.08 | 1334.83 |
| $\omega_7$ | 2.78 | 1.37 | -0.09 | 0.04 | -0.01 | 0.97 | 0.00 | 0.51 | -0.02 | 1154.79 |
| $\omega_8$ | 2.30 | 1.02 | -0.10 | 0.04 | -0.02 | 0.66 | 0.00 | 0.37 | -0.01 | 926.84 |
| $\omega_9$ | -0.42 | 0.69 | -0.10 | -0.06 | -0.08 | 0.67 | -0.17 | 0.28 | -0.18 | 685.61 |
| $\omega_{10}$ | 2.37 | 0.69 | 0.00 | 0.03 | 0.02 | 0.50 | -0.02 | 0.17 | 0.05 | 431.03 |
| $\omega_{11}$ | 2.87 | 0.31 | 0.13 | 0.11 | 0.12 | -0.06 | 0.11 | 0.06 | 0.23 | 248.62 |
| $\omega_{12}$ | 3.02 | 1.06 | -0.10 | 0.05 | -0.01 | 1.11 | 0.01 | 0.61 | -0.04 | 3128.55 |
| $\omega_{13}$ | 3.29 | 1.51 | -0.14 | 0.11 | 0.03 | 1.75 | 0.03 | 0.84 | -0.02 | 3033.59 |
| $\omega_{14}$ | 2.34 | 1.28 | -0.09 | 0.12 | 0.05 | 1.89 | 0.00 | 0.79 | -0.05 | 2956.18 |
| $\omega_{15}$ | 1.80 | 1.15 | -0.08 | 0.01 | -0.02 | 0.80 | -0.01 | 0.42 | -0.02 | 1496.69 |
| $\omega_{16}$ | 1.02 | 1.06 | -0.14 | 0.01 | -0.04 | 0.91 | -0.05 | 0.41 | -0.06 | 1412.96 |
| $\omega_{17}$ | 1.69 | 1.51 | -0.17 | -0.01 | -0.06 | 1.10 | -0.06 | 0.54 | -0.08 | 1341.78 |
| $\omega_{18}$ | 2.22 | 1.24 | -0.12 | 0.02 | -0.04 | 0.76 | -0.02 | 0.46 | -0.04 | 1174.61 |
| $\omega_{19}$ | 2.15 | 0.96 | -0.02 | 0.05 | 0.02 | 0.69 | 0.04 | 0.37 | 0.02 | 992.33 |
| $\omega_{20}$ | -1.09 | 0.57 | -0.13 | -0.10 | -0.11 | 0.86 | -0.17 | 0.29 | -0.17 | 718.55 |
| $\omega_{21}$ | 1.98 | 0.27 | 0.07 | 0.11 | 0.10 | 0.00 | 0.14 | 0.08 | 0.13 | 221.90 |

Table II: $g$-DMC: Harmonic vibrational frequencies.

| | (T) | T | (Q) | (Q)/A | (Q)/B | Q-1a | Q-1b | Q-3 | CC4 | Q |
|---|---|---|---|---|---|---|---|---|---|---|
| $A_e$ | 0.08% | 0.08% | -0.02% | 0.00% | -0.01% | 0.07% | -0.01% | 0.04% | -0.01% | 42792.3 |
| $B_e$ | 0.07% | 0.02% | 0.00% | 0.00% | 0.00% | 0.01% | 0.00% | 0.01% | 0.00% | 9494.5 |
| $C_e$ | 0.07% | 0.03% | 0.00% | 0.00% | 0.00% | 0.02% | 0.00% | 0.01% | 0.00% | 8458.3 |
| $r_{\mathrm{CC1}}$ | -0.0004 | -0.0002 | 0.0000 | 0.0000 | 0.0000 | -0.0001 | 0.0000 | -0.0001 | 0.0000 | 1.5198 |
| $r_{\mathrm{CC2}}$ | -0.0008 | -0.0007 | 0.0002 | 0.0000 | 0.0001 | -0.0005 | 0.0000 | -0.0003 | 0.0001 | 1.4139 |
| $r_{\mathrm{CH1}}$ | -0.0002 | -0.0001 | 0.0000 | 0.0000 | 0.0000 | -0.0001 | 0.0000 | -0.0001 | 0.0000 | 1.1061 |
| $r_{\mathrm{CH2}}$ | -0.0002 | -0.0001 | 0.0000 | 0.0000 | 0.0000 | -0.0001 | 0.0000 | 0.0000 | 0.0000 | 1.0982 |
| $r_{\mathrm{CH3}}$ | -0.0001 | -0.0001 | 0.0000 | 0.0000 | 0.0000 | -0.0001 | 0.0000 | -0.0001 | 0.0000 | 1.0953 |
| $r_{\mathrm{CH4}}$ | -0.0002 | -0.0001 | 0.0000 | 0.0000 | 0.0000 | -0.0002 | 0.0000 | -0.0001 | 0.0000 | 1.1055 |
| $r_{\mathrm{CH5}}$ | -0.0010 | -0.0010 | 0.0005 | 0.0001 | 0.0002 | -0.0007 | 0.0001 | -0.0005 | 0.0002 | 1.3349 |
| $r_{\mathrm{CH6}}$ | -0.0002 | -0.0001 | 0.0000 | 0.0000 | 0.0000 | -0.0001 | 0.0000 | 0.0000 | 0.0000 | 1.1022 |
| $\angle_{\mathrm{CCC}}$ | 0.014 | 0.037 | -0.008 | -0.004 | -0.006 | 0.027 | -0.005 | 0.015 | -0.005 | 112.189 |
| $\angle_{\mathrm{CCH1}}$ | 0.003 | -0.006 | 0.001 | 0.002 | 0.001 | -0.001 | 0.001 | -0.001 | 0.002 | 116.158 |
| $\angle_{\mathrm{CCH2}}$ | 0.002 | -0.001 | 0.003 | 0.000 | 0.001 | -0.002 | 0.000 | -0.002 | 0.001 | 111.536 |
| $\angle_{\mathrm{CCH3}}$ | 0.009 | 0.010 | -0.003 | 0.000 | -0.001 | 0.005 | 0.000 | 0.003 | -0.001 | 119.637 |
| $\angle_{\mathrm{CCH4}}$ | -0.004 | 0.003 | -0.002 | -0.002 | -0.001 | 0.001 | -0.001 | 0.000 | -0.001 | 124.638 |
| $\angle_{\mathrm{CCH5}}$ | 0.027 | 0.069 | -0.029 | -0.011 | -0.017 | 0.028 | -0.010 | 0.024 | -0.013 | 55.270 |
| $\angle_{\mathrm{CCH6}}$ | -0.002 | 0.023 | -0.009 | -0.004 | -0.006 | 0.012 | -0.004 | 0.008 | -0.005 | 105.370 |
| $\phi_1$ | -0.003 | -0.022 | 0.008 | 0.003 | 0.004 | -0.012 | 0.003 | -0.007 | 0.004 | 126.431 |
| $\phi_2$ | 0.001 | -0.009 | 0.005 | 0.002 | 0.003 | -0.006 | 0.002 | -0.004 | 0.002 | -119.230 |
| $\phi_3$ | 0.050 | 0.009 | 0.010 | 0.007 | 0.008 | 0.015 | 0.003 | 0.000 | 0.005 | 6.826 |
| $\phi_4$ | 0.051 | 0.048 | -0.020 | -0.006 | -0.010 | 0.016 | -0.004 | 0.016 | -0.006 | 176.960 |
| $\phi_5$ | -0.016 | 0.001 | 0.008 | -0.002 | 0.001 | -0.002 | -0.001 | -0.004 | -0.001 | 4.161 |
| $\phi_6$ | -0.056 | 0.023 | -0.028 | -0.013 | -0.017 | 0.007 | -0.011 | 0.012 | -0.014 | 99.937 |

Table III: $g$-TS: Geometry.

| | (T) | T | (Q) | (Q)/A | (Q)/B | Q-1a | Q-1b | Q-3 | CC4 | Q |
|---|---|---|---|---|---|---|---|---|---|---|
| $\omega_1$ | 2.55 | 1.24 | -0.16 | 0.05 | -0.04 | 1.50 | -0.07 | 0.72 | -0.12 | 3157.21 |
| $\omega_2$ | 2.49 | 1.03 | -0.14 | -0.04 | -0.08 | 0.96 | -0.06 | 0.55 | -0.11 | 3120.32 |
| $\omega_3$ | 2.56 | 1.16 | -0.19 | -0.05 | -0.10 | 1.14 | -0.08 | 0.62 | -0.13 | 3080.83 |
| $\omega_4$ | 3.98 | 1.94 | -0.30 | 0.24 | 0.03 | 2.63 | 0.00 | 1.17 | -0.05 | 2999.15 |
| $\omega_5$ | 2.65 | 1.21 | -0.15 | 0.01 | -0.05 | 1.62 | -0.07 | 0.75 | -0.13 | 2981.60 |
| $\omega_6$ | 5.01 | 1.11 | -0.23 | 0.36 | 0.16 | 2.05 | 0.27 | 0.89 | 0.19 | 2208.35 |
| $\omega_7$ | 1.83 | 1.70 | -0.28 | -0.05 | -0.13 | 1.23 | -0.10 | 0.65 | -0.14 | 1515.05 |
| $\omega_8$ | 1.39 | 1.05 | -0.09 | -0.04 | -0.05 | 0.67 | -0.05 | 0.36 | -0.06 | 1496.44 |
| $\omega_9$ | 1.32 | 1.14 | -0.16 | -0.07 | -0.09 | 0.70 | -0.07 | 0.39 | -0.09 | 1470.44 |
| $\omega_{10}$ | 1.75 | 1.49 | -0.25 | -0.04 | -0.11 | 1.08 | -0.07 | 0.55 | -0.11 | 1390.87 |
| $\omega_{11}$ | 3.27 | 2.42 | -0.55 | -0.02 | -0.19 | 1.84 | -0.08 | 0.96 | -0.17 | 1383.33 |
| $\omega_{12}$ | 2.79 | 2.20 | -0.41 | 0.07 | -0.08 | 1.76 | -0.01 | 0.95 | -0.07 | 1308.26 |
| $\omega_{13}$ | 1.67 | 1.41 | -0.19 | -0.04 | -0.09 | 1.00 | -0.06 | 0.55 | -0.09 | 1165.97 |
| $\omega_{14}$ | 2.00 | 1.26 | -0.18 | 0.01 | -0.06 | 1.03 | -0.01 | 0.52 | -0.03 | 1052.90 |
| $\omega_{15}$ | 1.46 | 1.19 | -0.21 | -0.04 | -0.10 | 0.85 | -0.06 | 0.46 | -0.08 | 1024.91 |
| $\omega_{16}$ | 1.77 | 1.26 | -0.18 | -0.01 | -0.07 | 0.89 | -0.03 | 0.49 | -0.05 | 1005.94 |
| $\omega_{17}$ | 1.70 | 1.22 | -0.17 | -0.03 | -0.09 | 0.89 | -0.05 | 0.50 | -0.07 | 907.19 |
| $\omega_{18}$ | 1.34 | 0.93 | -0.19 | -0.02 | -0.07 | 0.67 | -0.02 | 0.37 | -0.05 | 605.30 |
| $\omega_{19}$ | 0.73 | 0.35 | -0.05 | 0.01 | -0.01 | 0.31 | -0.01 | 0.13 | -0.01 | 434.60 |
| $\omega_{20}$ | 0.45 | -0.28 | 0.15 | 0.09 | 0.11 | -0.20 | 0.10 | -0.06 | 0.12 | 160.23 |
| $\omega_{21}$ | -7.82$i$ | 0.54$i$ | -0.44$i$ | -1.31$i$ | -1.08$i$ | -0.51$i$ | -1.11$i$ | 0.36$i$ | -0.78$i$ | 1169.16$i$ |

Table IV: $g$-TS: Harmonic vibrational frequencies.

| | (T) | T | (Q) | (Q)/A | (Q)/B | Q-1a | Q-1b | Q-3 | CC4 | Q |
|---|---|---|---|---|---|---|---|---|---|---|
| $A_e$ | 0.05% | 0.05% | -0.01% | -0.01% | -0.01% | 0.03% | -0.01% | 0.02% | -0.01% | 45867.5 |
| $B_e$ | 0.06% | 0.03% | -0.01% | 0.00% | 0.00% | 0.02% | 0.00% | 0.01% | 0.00% | 9174.1 |
| $C_e$ | 0.06% | 0.04% | -0.01% | 0.00% | -0.01% | 0.02% | 0.00% | 0.01% | 0.00% | 8028.2 |
| $r_{\mathrm{CC1}}$ | -0.0003 | -0.0001 | 0.0000 | 0.0000 | 0.0000 | -0.0001 | 0.0000 | -0.0001 | 0.0000 | 1.5096 |
| $r_{\mathrm{CC2}}$ | -0.0007 | -0.0006 | 0.0001 | 0.0001 | 0.0001 | -0.0003 | 0.0001 | -0.0002 | 0.0001 | 1.3488 |
| $r_{\mathrm{CH1}}$ | -0.0002 | -0.0001 | 0.0000 | 0.0000 | 0.0000 | -0.0001 | 0.0000 | 0.0000 | 0.0000 | 1.0981 |
| $r_{\mathrm{CH2}}$ | -0.0002 | -0.0001 | 0.0000 | 0.0000 | 0.0000 | -0.0001 | 0.0000 | 0.0000 | 0.0000 | 1.1000 |
| $r_{\mathrm{CH3}}$ | -0.0001 | -0.0001 | 0.0000 | 0.0000 | 0.0000 | -0.0001 | 0.0000 | 0.0000 | 0.0000 | 1.0899 |
| $r_{\mathrm{CH4}}$ | -0.0001 | -0.0001 | 0.0000 | 0.0000 | 0.0000 | -0.0001 | 0.0000 | 0.0000 | 0.0000 | 1.0917 |
| $r_{\mathrm{CH5}}$ | 0.0000 | 0.0000 | 0.0000 | 0.0000 | 0.0000 | -0.0001 | 0.0000 | 0.0000 | 0.0000 | 1.0934 |
| $\angle_{\mathrm{CCC}}$ | 0.007 | 0.015 | -0.003 | -0.003 | -0.003 | 0.008 | -0.002 | 0.004 | -0.003 | 124.576 |
| $\angle_{\mathrm{CCH1}}$ | 0.001 | 0.007 | -0.001 | -0.001 | -0.001 | 0.006 | -0.001 | 0.003 | -0.001 | 111.103 |
| $\angle_{\mathrm{CCH2}}$ | -0.006 | -0.001 | -0.001 | -0.001 | -0.001 | -0.002 | -0.001 | 0.000 | -0.001 | 110.930 |
| $\angle_{\mathrm{CCH3}}$ | -0.004 | 0.002 | -0.001 | -0.001 | -0.001 | 0.000 | 0.000 | 0.000 | 0.000 | 121.465 |
| $\angle_{\mathrm{CCH4}}$ | 0.001 | 0.009 | -0.002 | -0.001 | -0.002 | 0.007 | -0.001 | 0.003 | -0.002 | 121.231 |
| $\angle_{\mathrm{CCH5}}$ | 0.001 | -0.013 | 0.003 | 0.003 | 0.003 | -0.008 | 0.002 | -0.003 | 0.003 | 116.539 |
| $\phi$ | 0.000 | 0.001 | 0.000 | 0.000 | 0.000 | 0.000 | 0.000 | 0.000 | 0.000 | 120.564 |

Table V: Propene: Geometry.

| | (T) | T | (Q) | (Q)/A | (Q)/B | Q-1a | Q-1b | Q-3 | CC4 | Q |
|---|---|---|---|---|---|---|---|---|---|---|
| $\omega_1$ | 1.49 | 0.85 | -0.30 | -0.17 | -0.23 | 0.89 | -0.20 | 0.53 | -0.25 | 3246.62 |
| $\omega_2$ | 1.44 | 0.88 | -0.35 | -0.19 | -0.26 | 1.12 | -0.27 | 0.55 | -0.33 | 3164.79 |
| $\omega_3$ | 1.51 | 0.83 | -0.27 | -0.12 | -0.18 | 1.14 | -0.20 | 0.57 | -0.23 | 3148.29 |
| $\omega_4$ | 2.41 | 0.95 | -0.20 | -0.09 | -0.14 | 0.83 | -0.14 | 0.48 | -0.18 | 3131.08 |
| $\omega_5$ | 1.88 | 0.33 | -0.53 | -0.42 | -0.46 | 0.73 | -0.48 | 0.11 | -0.53 | 3036.84 |
| $\omega_6$ | 4.12 | 4.41 | -0.46 | -0.19 | -0.26 | 2.11 | 0.00 | 1.56 | -0.13 | 1689.12 |
| $\omega_7$ | 1.12 | 0.85 | -0.15 | -0.12 | -0.13 | 0.47 | -0.11 | 0.24 | -0.13 | 1499.98 |
| $\omega_8$ | 1.18 | 1.23 | -0.20 | -0.14 | -0.16 | 0.70 | -0.14 | 0.41 | -0.15 | 1449.62 |
| $\omega_9$ | 1.13 | 1.13 | -0.16 | -0.10 | -0.12 | 0.71 | -0.12 | 0.38 | -0.12 | 1408.89 |
| $\omega_{10}$ | 0.74 | 0.86 | -0.86 | -0.76 | -0.80 | 0.21 | -0.69 | -0.10 | -0.75 | 1315.11 |
| $\omega_{11}$ | 1.07 | 1.04 | -0.16 | -0.10 | -0.13 | 0.57 | -0.10 | 0.36 | -0.12 | 1188.27 |
| $\omega_{12}$ | 0.81 | 0.75 | -0.12 | -0.07 | -0.09 | 0.51 | -0.09 | 0.27 | -0.10 | 939.59 |
| $\omega_{13}$ | 1.02 | 0.80 | -0.12 | -0.06 | -0.08 | 0.54 | -0.05 | 0.34 | -0.07 | 925.96 |
| $\omega_{14}$ | 0.59 | 0.51 | -0.06 | -0.03 | -0.04 | 0.32 | -0.03 | 0.19 | -0.05 | 416.12 |
| $\omega_{15}$ | 2.70 | 0.94 | -0.12 | -0.03 | -0.06 | 0.98 | -0.04 | 0.52 | -0.08 | 3107.44 |
| $\omega_{16}$ | 1.17 | 0.89 | -0.08 | -0.06 | -0.07 | 0.51 | -0.06 | 0.28 | -0.07 | 1487.74 |
| $\omega_{17}$ | 1.46 | 1.26 | -0.19 | -0.14 | -0.16 | 0.68 | -0.11 | 0.38 | -0.12 | 1066.03 |
| $\omega_{18}$ | 2.76 | 1.99 | -0.27 | -0.22 | -0.23 | 0.97 | -0.10 | 0.58 | -0.12 | 1008.20 |
| $\omega_{19}$ | 2.99 | 2.71 | -0.41 | -0.24 | -0.27 | 1.59 | -0.10 | 0.88 | -0.14 | 908.76 |
| $\omega_{20}$ | 1.33 | 1.09 | -0.17 | -0.14 | -0.15 | 0.57 | -0.09 | 0.32 | -0.10 | 575.64 |
| $\omega_{21}$ | 0.52 | 0.27 | -0.04 | -0.04 | -0.04 | 0.00 | -0.01 | 0.06 | -0.01 | 200.80 |

Table VI: Propene: Harmonic vibrational frequencies.

| | (T) | T | (Q) | (Q)/A | (Q)/B | Q-1a | Q-1b | Q-3 | CC4 | Q |
|---|---|---|---|---|---|---|---|---|---|---|
| $A_e$ | 0.55% | 0.38% | -1.38% | 0.67% | -0.58% | 0.64% | 0.11% | 0.16% | -0.05% | 75323.7 |
| $B_e$ | 0.21% | 0.20% | -0.31% | 0.01% | -0.20% | 0.14% | -0.01% | 0.08% | -0.03% | 12200.9 |
| $C_e$ | 0.26% | 0.23% | -0.46% | 0.11% | -0.26% | 0.21% | 0.00% | 0.09% | -0.03% | 10500.1 |
| $r_{\mathrm{OO}}$ | -0.0042 | 0.0012 | 0.0051 | -0.0026 | 0.0040 | 0.0001 | -0.0001 | -0.0005 | -0.0004 | 1.3628 |
| $r_{\mathrm{CO}}$ | -0.0007 | -0.0052 | 0.0049 | -0.0008 | 0.0009 | -0.0046 | -0.0002 | -0.0011 | 0.0009 | 1.2910 |
| $r_{\mathrm{CH1}}$ | 0.0001 | 0.0003 | -0.0001 | -0.0005 | -0.0003 | -0.0002 | -0.0001 | -0.0001 | -0.0001 | 1.0887 |
| $r_{\mathrm{CH2}}$ | -0.0001 | 0.0003 | 0.0000 | -0.0006 | -0.0002 | -0.0002 | -0.0001 | -0.0001 | -0.0001 | 1.0864 |
| $\angle_{\mathrm{OOC}}$ | 0.145 | 0.041 | -0.396 | 0.237 | -0.163 | 0.158 | 0.039 | 0.028 | -0.005 | 117.416 |
| $\angle_{\mathrm{OCH1}}$ | 0.019 | 0.030 | -0.014 | 0.078 | 0.042 | 0.060 | 0.010 | 0.006 | -0.002 | 119.082 |
| $\angle_{\mathrm{OCH2}}$ | 0.024 | 0.151 | -0.075 | -0.066 | -0.042 | 0.064 | -0.018 | 0.018 | -0.037 | 115.005 |

Table VII: CI: Geometry.

| | (T) | T | (Q) | (Q)/A | (Q)/B | Q-1a | Q-1b | Q-3 | CC4 | Q |
|---|---|---|---|---|---|---|---|---|---|---|
| $\omega_1$ | 1.31 | -2.86 | 0.11 | 6.23 | 2.59 | 2.62 | 1.40 | 0.85 | 0.90 | 3325.12 |
| $\omega_2$ | 2.10 | -1.37 | -0.10 | 6.03 | 2.64 | 3.56 | 1.32 | 1.10 | 0.82 | 3162.27 |
| $\omega_3$ | 0.47 | 8.55 | -7.66 | 2.75 | -1.41 | 7.85 | 0.41 | 1.88 | -1.46 | 1467.90 |
| $\omega_4$ | -12.36 | 26.98 | -19.75 | 0.18 | -3.63 | 21.85 | 1.22 | 4.55 | -4.84 | 1262.46 |
| $\omega_5$ | 5.13 | 3.51 | -8.64 | 2.99 | -3.93 | 3.27 | 0.20 | 1.18 | -0.50 | 1213.24 |
| $\omega_6$ | 33.75 | -10.52 | 6.60 | -5.18 | -15.37 | -18.44 | -2.51 | -1.92 | 2.77 | 885.75 |
| $\omega_7$ | 2.37 | -0.36 | -3.47 | 2.58 | -2.39 | 0.21 | 0.12 | 0.43 | 0.13 | 524.59 |
| $\omega_8$ | 8.51 | 30.08 | -23.18 | -2.73 | -6.94 | 22.99 | 0.62 | 6.23 | -4.05 | 794.23 |
| $\omega_9$ | 0.73 | 8.63 | -15.37 | 1.73 | -5.89 | 9.27 | 1.47 | 2.50 | -1.08 | 607.90 |

Table VIII: CI: Harmonic vibrational frequencies.
